# Supplementary material for: ReconVAT: A Semi-Supervised Automatic Music Transcription Framework for Low-Resource Real-World Data
Source: arXiv:2107.04954 source file (2021-07-29)
Supplement: Supplementary file 1 [file Appendix.tex]

\onecolumn
\section{Appendix}

\subsection{MusicNet Splitting}
This section contains two tables that describe the labelled training, unlabelled training, and test split for the MusicNet dataset.
\begin{table*}[hbt!]
  \caption{The training and test split for the string version of MusicNet.}
  \label{tab:string_data}
  \begin{tabular}{P{3cm}P{1.5cm}P{7.2cm}P{1.5cm}}
    \toprule
    Genre & Labelled Train ID & Unlabelled Train ID & Test ID\\
    \midrule
    Solo violin & 2186 & 2241, 2242, 2243, 2244, 2288, 2289, 2659 & 2191\\\hline
    Violin and harpsichord & 2282 & 2283, 2284, 2285 & N.A.\\\hline
    Accompanied violin & 2330 & 2334, 2335, 2336, 2341, 2342, 2397, 2398, 2420, 2462, 2463, 2466,
      2501, 2502, 2570, 2571, 2572, 2573, 2626, 2627, 2629 & 2628\\\hline
    String quartet & 1788 & 1789, 1790, 1791, 1792, 1793, 1805, 1807, 1822, 1824, 1835, 1859,
      1916, 1918, 1919, 1922, 1923, 1931, 1932, 1933, 2104, 2105, 2138,
      2140, 2177, 2178, 2179, 2180, 2313, 2314, 2315, 2365, 2366, 2368,
      2376, 2377, 2379, 2381, 2383, 2384, 2403, 2431, 2432, 2433, 2451,
      2480, 2481, 2482, 2483, 2494, 2497, 2560, 2562, 2621, 2622 & 2106\\\hline
    String sextet & 2147 & 2154, 2155, 2156, 2157 & N.A.\\\hline
    Viola Quintet & 1742 & N.A. & N.A.\\\hline
    Solo cello & 2217 & 2218, 2219, 2220, 2221, 2222, 2293, 2294, 2295, 2296, 2297 & 2298\\\hline
    Accompanied Cello & 2112 & 2113, 2114, 2521, 2522, 2523, 2586 & N.A.\\\hline
  \bottomrule
  Total number & 8 & 104 & 4
\end{tabular}
\end{table*}
\begin{table*}[hbt!]
  \caption{The training and test split for the woodwind version of MusicNet.}
  \label{tab:woodwind_data}
  \begin{tabular}{P{3cm}P{1.5cm}P{7.2cm}P{1.5cm}}
    \toprule
    Genre & Labelled Train ID & Unlabelled Train ID & Test ID\\
    \midrule
    Accompanied Clarinet & 2116 & 2117, 2118, 2119 & N.A.\\\hline
    Clarinet Quintet & 1811 & 1812, 1813 & N.A.\\\hline
    Pairs Clarinet-Horn-Bassoon & 1817 & 1818, 2415, 2417 & 1819, 2416\\\hline
    Clarinet-Cello-Piano Trio & 2318 & 2319, 2320 & N.A.\\\hline
    Wind Octet & 2504 & 2505, 2506, 2507 & N.A.\\\hline
    Wind Quintet & 2075 & 2076, 2077, 2078, 2079, 2080, 2081, 2082, 2083 & N.A.\\\hline
  \bottomrule
  Total number & 6 & 21 & 2
\end{tabular}
\end{table*}

\subsection{Transcription Examples and Audio Samples}
To get access to more transcription results and listen to the audio examples, readers are referred to our demo page at https://kinwaicheuk.github.io/ReconVAT.
